# Supplementary material for: JanusAQP: Efficient Partition Tree Maintenance for Dynamic Approximate Query Processing
Source: arXiv:2204.09235 source file (2022-07-26)
Supplement: Supplementary file 1 [file additionals.tex]

In this section we propose new algorithms for constructing a partition over the samples items $\samples$. Our algorithms can be used in different scenarios: i) construct a partition the first time over $\samples$, ii) construct a new partition if the re-partition is needed after a number of updates in our dataset, and iii) check if repartition is needed after an insertion or deletion of an item, i.e., is there a partition with significantly less error than the current partition?
%In the end of this section we formally describe how Dynamic PASS decides when a re-partition/re-construction of $\PASStree$ is needed.

In~\cite{liang2021combining} the authors proposed algorithms for constructing near optimal partitions.
However, most their algorithms run in time roughly $O(km\log m)$. For the offline version of the problem their algorithm is very efficient since it is linear in both parameters $k, m$. Ideally, in the dynamic setting, we do not want the update procedure to depend linearly on $m$, i.e., the number of samples we store. Here we design data structures and algorithms that run the re-partition (or the check if there is a better partition) in only $O(k)$ time, ignoring $\polylog$ factors, which is near-optimal since we have $k$ buckets.

In order to achieve faster algorithms we propose new dynamic data structures for various sub-problems. Mainly, we propose an efficient dynamic data structures such that given a query rectangle, it returns (approximately) the maximum variance of a query completely inside the query rectangle. Using this data structure, we can achieve a very fast construction of $\PASStree$ in any dimension $d$.
For $d=1$ we manage to design a very efficient algorithm making an assumption on the aggregation values of the items. In particular we assume that the values of items are bounded by a polynomial on $N$, i.e. the total number of items in the full dataset. This is usually the case in real datasets so it is not a strong assumption and it is made in several papers~\cite{guha2006approximation} for constructing histograms with low error. %We notice that the assumption is not needed in higher dimensions.

We start by introducing some basic notation and by defining some basic notions. Then we describe our new dynamic data structures for finding maximum error queries.
We continue by presenting the partition algorithm for $d=1$ and the partition algorithm for any dimension $d>1$.
In the end of this section we show an algorithm to decide when re-partition is needed.

\subsection{Preliminaries}
The goal of \sys is to construct a dynamic partition tree $\PASStree$ such that the maximum error (confidence interval) of a query is minimized. Recall that the leaf nodes of $\PASStree$ define a partition over the samples $\samples$.
As we discussed in previous sections the number of samples $H$ (catch-up phase) is going to be much larger than the number of samples in $\samples$. In particular, the sampling rate of $H$ in the end of the catch-up phase is significantly higher than the sampling rate of $\samples$ we store in $\PASStree$. Hence we expect that the error (variance) of nodes in $U_2$ will be much lower comparing to the error of the nodes in $U_1$ for a query $q$. So we focus on finding a partition that minimizes the longest confidence interval of any possible query considering only the error from the leaf nodes that partially intersect the query.

As shown in~\cite{liang2021combining}, in order to find the query with the worst confidence interval in the partition defined by the leaf nodes of $\PASStree$, it is sufficient to consider only queries that lie completely inside the leaf nodes of $\PASStree$.
Indeed by considering only these queries we can still get a $\sqrt{k}$-approximation for COUNT and SUM queries over the optimum partition considering all queries. The approximation factor improves to $\sqrt{2}$ for $d=1$. For AVG queries the error of the optimum partition considering queries completely inside the leaf nodes is the same with the maximum error considering every possible query. So without loss of generality we solve the optimization problem of finding a partition that minimizes the maximum error considering only queries that lie completely inside the buckets of a partition.

%Static PASS~\cite{hellerstein2008quantitative} tries to find a tree structure such that its leaf nodes define a partition over the samples $\samples$ to (approximately) minimize the length of the longest confidence interval. Equivalently, in PASS they are trying to find a partition that minimizes the maximum error. The authors in~\cite{liang2021combining} argue that instead of looking over all possible queries to minimize the maximum error they focus on queries that lie completely inside one bucket. Indeed, the optimum partition considering only queries that lie completely inside a bucket has error at most $\sqrt{k}$ times more than the error over the optimum partition for COUNT/SUM queries. For AVG queries the error of the optimum partition considering queries completely inside buckets is the same with the maximum error considering every possible query.

%Similarly to~\cite{liang2021combining}, considering only queries completely inside a bucket gives a $\sqrt{k}$ approximation for COUNT/SUM queries and $1$-approximation (optimum) for AVG queries. For $1$D it gives a $\sqrt{2}$ approximation for COUNT/SUM queries.

Let $u$ be a leaf node of $\PASStree$ and let $q$ be a query completely inside $R_u$. In this case notice that $w_u=1$ for all types of queries.
From Section~\ref{sec:estimators}, recall that the variance of any COUNT or SUM query completely inside $R_u$ has a factor $\frac{N_u^2}{m_u^2}$. This factor is the same in all queries inside $u$ so without loss of generality we can skip it from the variance definition (considering queries inside $R_u$).
Furthermore, notice that the confidence interval of any query inside $R_u$ has a factor $\frac{1}{m_u}$ which is also the same. Hence, the problem of finding the query with the largest confidence interval in $u$ is equivalent with the problem of finding the query $q$ in $u$ that maximizes the following function.
If $q$ is a COUNT or SUM query:
$$\nu_s(q)=m_u\sum_{t\in q}t.a^2-\left(\sum_{t\in q}t.a\right)^2,$$
and if $q$ is an AVG query:
$$\nu_s(q)=\frac{1}{|q|^2}\left[m_u\sum_{t\in q}t.a^2-\left(\sum_{t\in q}t.a\right)^2\right].$$

In order to make sure that we return accurate estimators we require that each bucket contains a sufficiently large amount of samples, roughly $\Omega(\frac{1}{\alpha}\log m)$ samples, where $\alpha$ is the sampling rate of $\samples$.
%If that holds, it is known from~\cite{liang2021combining} that with high probability the ratio $\frac{N_u}{m_u}$ for any possible leaf node $u$ will be within a constant factor from the ratio $N/m$, so it will be almost the same for any bucket we construct.
Furthermore, we study queries that contain at least $\delta m$ samples from each bucket that they partially intersect, for a small parameter $\delta<1$. Otherwise a query does not include many samples and we are not be able to return an accurate estimator along with a provable confidence interval. We note that these assumptions were also made in~\cite{liang2020fast}.
%Finally, we define the following notation which is useful in the next subsections. For a rectangle $R$, let $\optVar(R)$ be the variance of the query with the maximum variance in $R$.
